# Supplementary material for: Superfluidic nature of self-driven nanofluidics at liquid-gas interfaces
Source: arXiv:2208.13759 source file (2022-08-31)
Supplement: Supplementary file 1 [file SI.tex]

\maketitle

\section{Notations}
\begin{table}[h!]
\begin{tabular}{ l  l }
\hline
 $\sigma$& Position of nanopore from the reference edge \\
 $d$& Diameter of the Nanopore
\\
 $\gamma$& Phase volume fraction in the multiphase flow\\
 $\rho$& Phase density\\
 $\kappa$& Phase variable\\
 $\bm v_p$& Phase velocity\\
 $\bm v_g$& group velocity\\
 $k$& Wave number\\
 $a$& Acceleration of the molecules\\
 $N$& Number of particles in the system\\
 $k_B$& Boltzmann constant\\
 $\Gamma$& Cross sectional area\\
 $P$& Pressure\\
 $\eta$& Viscosity of liquid\\
 $L$& Flow length of instability\\
 $\alpha_{e}$& Element size in the simulation\\
 $N_{e}$& Number of elements in simulation\\
 $\Phi$& Area of nanopore\\
 $\bm{r}$& Position vector\\
 $b$& Distance constant\\
 $\bm{\beta}$& Constant velocity component in a vortex pair\\
 $(u, v, w)$& Velocity components in $x, y, z$ direction\\
 $R_e$& Reynolds number\\
  $E$& Energy\\
 $k_{eff}$& Effective thermal conductivity\\
 suffix $_{g, l}$& Gas phase and liquid phase, respectively\\
 suffix $_{a, s}$& Analytical and simulation, respectively\\
 suffix $_{in}$& Interface\\
 $\zeta$ & finite range interactos between particles\\
 $\bm v_c$ & critical velocity\\
 \bm{p_c} & critical momentum\\
 \bm{q} & condensate momentum\\
 \tau & constant corresponding to equation 1 \\
 E & Reletivistic energy\\
 B & Wave amplitude\\
 \varphi^$\dagger$ & creation operator\\
 \varphi & annihilation operator\\
 \phi_b & quantum state of system before interaction\\
 $\phi_{\chi}$ & quantum state of system after interaction\\
\hline
\end{tabular}
\end{table}
\newpage
